# Supplementary material for: A Simple Recipe for Competitive Low-compute Self supervised Vision Models
Source: arXiv:2301.09451 source file (2023-01-23)
Supplement: Supplementary file 1 [file low_shot_more.tex]

\begin{table}[]
    \centering
    \begin{tabular}{c |l l c| c}
        Arch & Method & Teacher & GFlops & IN-$1\%$ \\
        \midrule
        % \multicolumn{4}{l}{\small\bf\it Self-supervised distillation}\\
        RN18 & SEED & MoCoV2 RN152 & 11.6 & 44.3 \\
        RN18 & DisCo & MoCoV2 RN152 & 11.6 & 47.1 \\
        RN18 & BINGO & SwAV RN50x2 & 16.2 & 48.2 \\
        RN18 & BINGO & MoCoV2 RN152 & 11.6 & \underline{50.3} \\
        \midrule
        RN18 & RoB & SwAV RN50 & 4.1 & 46.3 \\
        RN18 & RoB & SwAV RG128 & 127.9 & 47.3 \\
        RN18 & RoB & DINO-S/8 & 22.4 & 47.8 \\
        \midrule
        RN34 & RoB & SwAV RN50 & 4.1 & 53.5 \\
        RN34 & RoB & SwAV RG128 & 127.9 & 54.9 \\
        RN34 & RoB & DINO-S/8 & 22.4 & 55.5 \\
        \midrule
        ViT-Ti & RoB& DINO S/8 & 22.4 & 54.0 \\
        ViT-Ti & RoB& iBOT L/16 & 61.6 & 56.2 \\
        ViT-Ti & RoB& MSN B/16 & 17.6 & \bf 58.7 \\
        \bottomrule
    \end{tabular}
    \caption{\textbf{Semi-supervised learning with RoB}, on ImageNet. All of our students trained with RoB, compared with each other and with other self-supervised distillation approaches. Evaluations follow the protocol described in Appendix~\ref{appendix:low_shot_protocol}.}
    \label{tab:msn_low_shot}
\end{table}
