# Supplementary material for: A Simple Recipe for Competitive Low-compute Self supervised Vision Models
Source: arXiv:2301.09451 source file (2023-01-23)
Supplement: Supplementary file 5 [file vit_s16_full.tex]

\begin{table*}[t]
    \centering
    \begin{tabular}{c|c c c|c c c c c c | c}
        Arch & Method & Teacher & Params & IN1K & iNat18 & Clevr/C & Clevr/D & Cifar100 & Places & Mean \\
        \midrule
        \multicolumn{10}{l}{\small\bf\it Methods without distillation}\\
        ViT-S/16 & DINO & - & - & 77.0 & 49.8 & 82.3 & 64.5 & 81.2 & 53.7 & 68.08 \\
        ViT-S/16 & iBOT & - & - & 77.0 & 48.9 & 85.7 & 65.5 & 81.4 & 53.9 & 68.73 \\
        \midrule
        \multicolumn{10}{l}{\small\bf\it Self-supervised distillation}\\
        ViT-S/16 & RoB (300ep) & DINO S/8 & 22M & 77.3 & 48.5 & 82.9 & 63.3 & 83.5 & 53.6 & \cc 68.18 \\
        ViT-S/16 & RoB (400ep) & iBOT L/16 & 305M & 78.2 & 46.5 & 85.6 & 65.5 & 82.0 & 54.8 & \cc 68.77 \\
        \bottomrule
    \end{tabular}
    \caption{\textbf{RoB with large students}. Trying RoB to produce stronger ViT-S/16 that if trained with DINO or iBOT alone. The students are of the same average performance as training without a teacher, which shows that RoB does not degrade performance, but RoB is mostly useful for students that cannot be efficiently trained with SSL in the first place.}
    \label{tab:large_students}
\end{table*}
